# Supplementary material for: SVRecon: Sparse Voxel Rasterization for Surface Reconstruction
Source: arXiv:2511.17364 source file (2025-11-21)
Supplement: Supplementary file 1 [file z_symbols.tex]

%%%%%%%%%%%%%%%%%%%%%%%%%%%%%%%%%%%%%%%%%%%%%%%%%%%%%%%%%%%%%%%%
% SH
%%%%%%%%%%%%%%%%%%%%%%%%%%%%%%%%%%%%%%%%%%%%%%%%%%%%%%%%%%%%%%%%
% \textbf{Symbol definition}
% We first define the symbols and notations used throughout the paper. 
% While voxels can be categorized into 'inside' and 'outside' regions, this paper focuses exclusively on the inside region, from which the mesh is extracted. 
% \textbf{Symbol Definitions}

% \textbf{Symbol Definitions}

We first define the symbols and notations used throughout the paper. To facilitate our explanations, we define the predefined cube region (length $D$) of interest using two distinct coordinate systems for convenience: (1) a dynamic dense coordinate $\mathbf{d}$, which depends on the current state of the octree, and (2) a static world coordinate $\mathbf{x}$.

1) General \& Grid Definitions

$L_{max}$: The maximum allowed subdivision level.

$L$: The maximum subdivision level present in the current octree.

$G = 2^L$: The grid resolution of the dense coordinate space at level $L$.

$\mathbf{d_L}=(i,j,k)\in\{0,\ldots,G-1\}^3$: A dense coordinate in the finest lattice (level $L$).

$\mathrm{idx}(i,j,k)=i\cdot G^2+j\cdot G+k$: The linearized dense index for a coordinate $(i,j,k)$.

2) Voxel Properties (in Dense Space)

$N_{vox}$: The total number of voxels in the current octree.

$v \in \mathcal{V},\; \mathcal{V}=\{0,\ldots,N_{vox}-1\}$: A voxel index.

$l_v \in [1,L]$: The subdivision level of voxel $v$.

$geo_v \in \mathbb{R}^{2\times 2\times 2}$: The geometric values stored at the eight corners of voxel $v$.

$rgb_v$ : color of voxel $v$ stored per voxel

$c_v \in \mathbb{R}^3$: The center coordinate of voxel $v$ in the dense coordinate space.

$h_v = 2^{L-l_v}$: The side length of voxel $v$ in the dense coordinate space (e.g., 1, 2, 4...).

$\mathbf{d}_{min}(v), \mathbf{d}_{max}(v)$: The min/max corner coordinates of voxel $v$ in dense space: $\mathbf{d}_{min}(v)=\mathbf{c_v}-0.5\times h_v$ and $\mathbf{d}_{max}(v)=\mathbf{c_v} + 0.5\times h_v$.

3) World Coordinate Mapping

$h_L = D/2^L$: The world coordinate length of a minimum-sized voxel (a single cell).

$\mathbf{x}(\mathbf{d_L})$: A mapping function from a dense coordinate $\mathbf{d_L}$ to its corresponding world coordinate $\mathbf{x}$. This is defined as:

$$\mathbf{x}(\mathbf{d_L}) \;=\; \mathbf{x}_{\min} \;+\; \frac{\mathbf{d_L}}{G}\,\odot\,(\mathbf{x}_{\max}-\mathbf{x}_{\min})$$

where $\mathbf{x}_{\min}$ and $\mathbf{x}_{\max}$ define the world-space boundaries of the region.
